# Supplementary material for: Traffic Simulations: Multi-City Calibration of Metropolitan Highway Networks
Source: arXiv:2501.04783 source file (2025-01-08)
Supplement: Supplementary file 1 [file 6_appendix.tex]

\begin{figure}[htb]
	\center
	\includegraphics[width=0.45\textwidth]{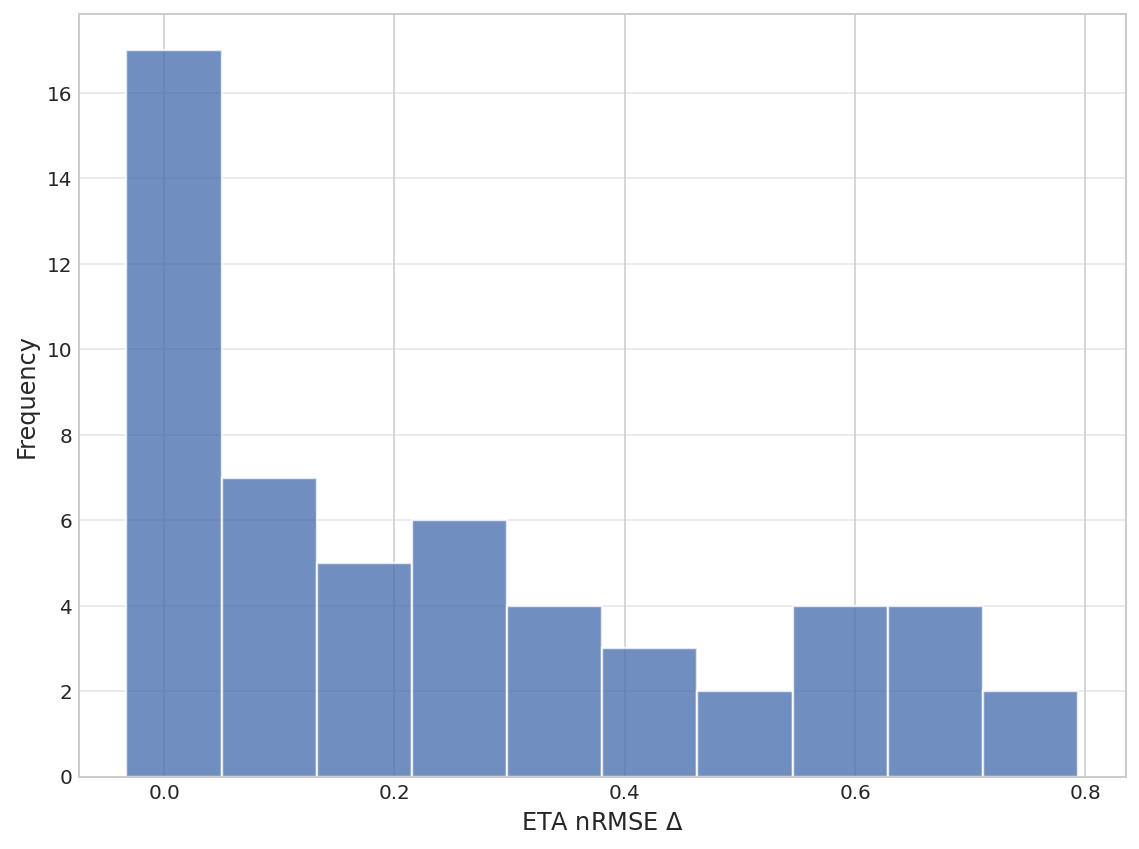}
    \caption{Distribution of relative improvement as measured by $\Delta$ in ETA nRMSE.}
    \label{fig:delta_histogram}
\end{figure}
